# Supplementary material for: Tailor: Size Recommendations for High-End Fashion Marketplaces
Source: arXiv:2401.01978 source file (2024-01-03)
Supplement: Supplementary file 1 [file appendix-model-hyperparameters.tex]

\begin{minipage}{.5\textwidth}
    \subsection{PMCV Hyper-parameters} \label{pmcv_hyperparameters}
    \begin{lstlisting}[style=yaml]
input_hierarchy:
    - ["user_id", "category_id", "brand_id"]
    - ["user_id", "cateogry_id"]
    - ["user_id", "brand_id"]
    - ["user_id"]
    - ["category_id", "brand_id"]
    - ["category_id"]
\end{lstlisting}
\end{minipage}% This must go next to `\end{minipage}`
\begin{minipage}{.5\textwidth}
    \subsection{SFNet Hyper-parameters}  \label{sfnet_hyperparameters}
    \begin{lstlisting}[style=yaml]
user_inputs:
    - "user_id",
product_inputs:
    - "brand_id"
    - "category_id"
    - "scale_id"
    - "product_id"
embedding_dim: 20
user_pathway_dims: [50, 30, 20]
item_pathway_dims: [50, 30, 20]
combined_pathway_dims: [100, 200, 400, 1000]
activation: "tanh"
dropout: 0.05
\end{lstlisting}
\end{minipage}

\begin{minipage}{.5\textwidth}
    \subsection{SSP-LSTM Hyper-parameters}  \label{ssp-lstm_hyperparameters}
    \begin{lstlisting}[style=yaml]
embeddings_parameters:
  brand_id:
    dim: 8
  category_id:
    dim: 4
  return_reason:
    dim: 2
  size_position:
    dim: 3
  scale_id:
    dim: 6
  event_type:
    dim: 2
BiLSTM:
  dropout: 0.01
  hidden_layer_size: 25
  number_layers: 2
ProductEncoder:
  activation: relu
  dropout: 0.01
  hidden_state_dimensions:
    - 50
    - 25
MixerEncoder:
  activation: relu
  dropout: 0.01
  hidden_state_dimensions:
    - 150
    - 100
\end{lstlisting}
\end{minipage}% This must go next to `\end{minipage}`
\begin{minipage}{.5\textwidth}
    \subsection{SSP-Attention Hyper-parameters}  \label{ssp-attention_hyperparameters}
    \begin{lstlisting}[style=yaml]
embeddings_parameters:
  brand_id:
    dim: 64
  category_id:
    dim: 48
  return_reason:
    dim: 2
  size_position:
    dim: 16
  scale_id:
    dim: 48
  event_type:
    dim: 2
TransformerBlock1:
  num_heads: 12
TransformerBlock2:
  num_heads: 16
MLP:
  activation: relu
  dropout: 0.01
  hidden_state_dimensions:
    - 150
    - 100
\end{lstlisting}

\end{minipage}
